# Supplementary material for: GACELA -- A generative adversarial context encoder for long audio inpainting
Source: arXiv:2005.05032 source file (2020-05-11)
Supplement: Supplementary file 1 [file supplementary_friedhof.tex]

\newpage

\section*{Supplementary Material}

\begin{figure*}[!th]
\begin{center}
	\includegraphics[width=\textwidth]{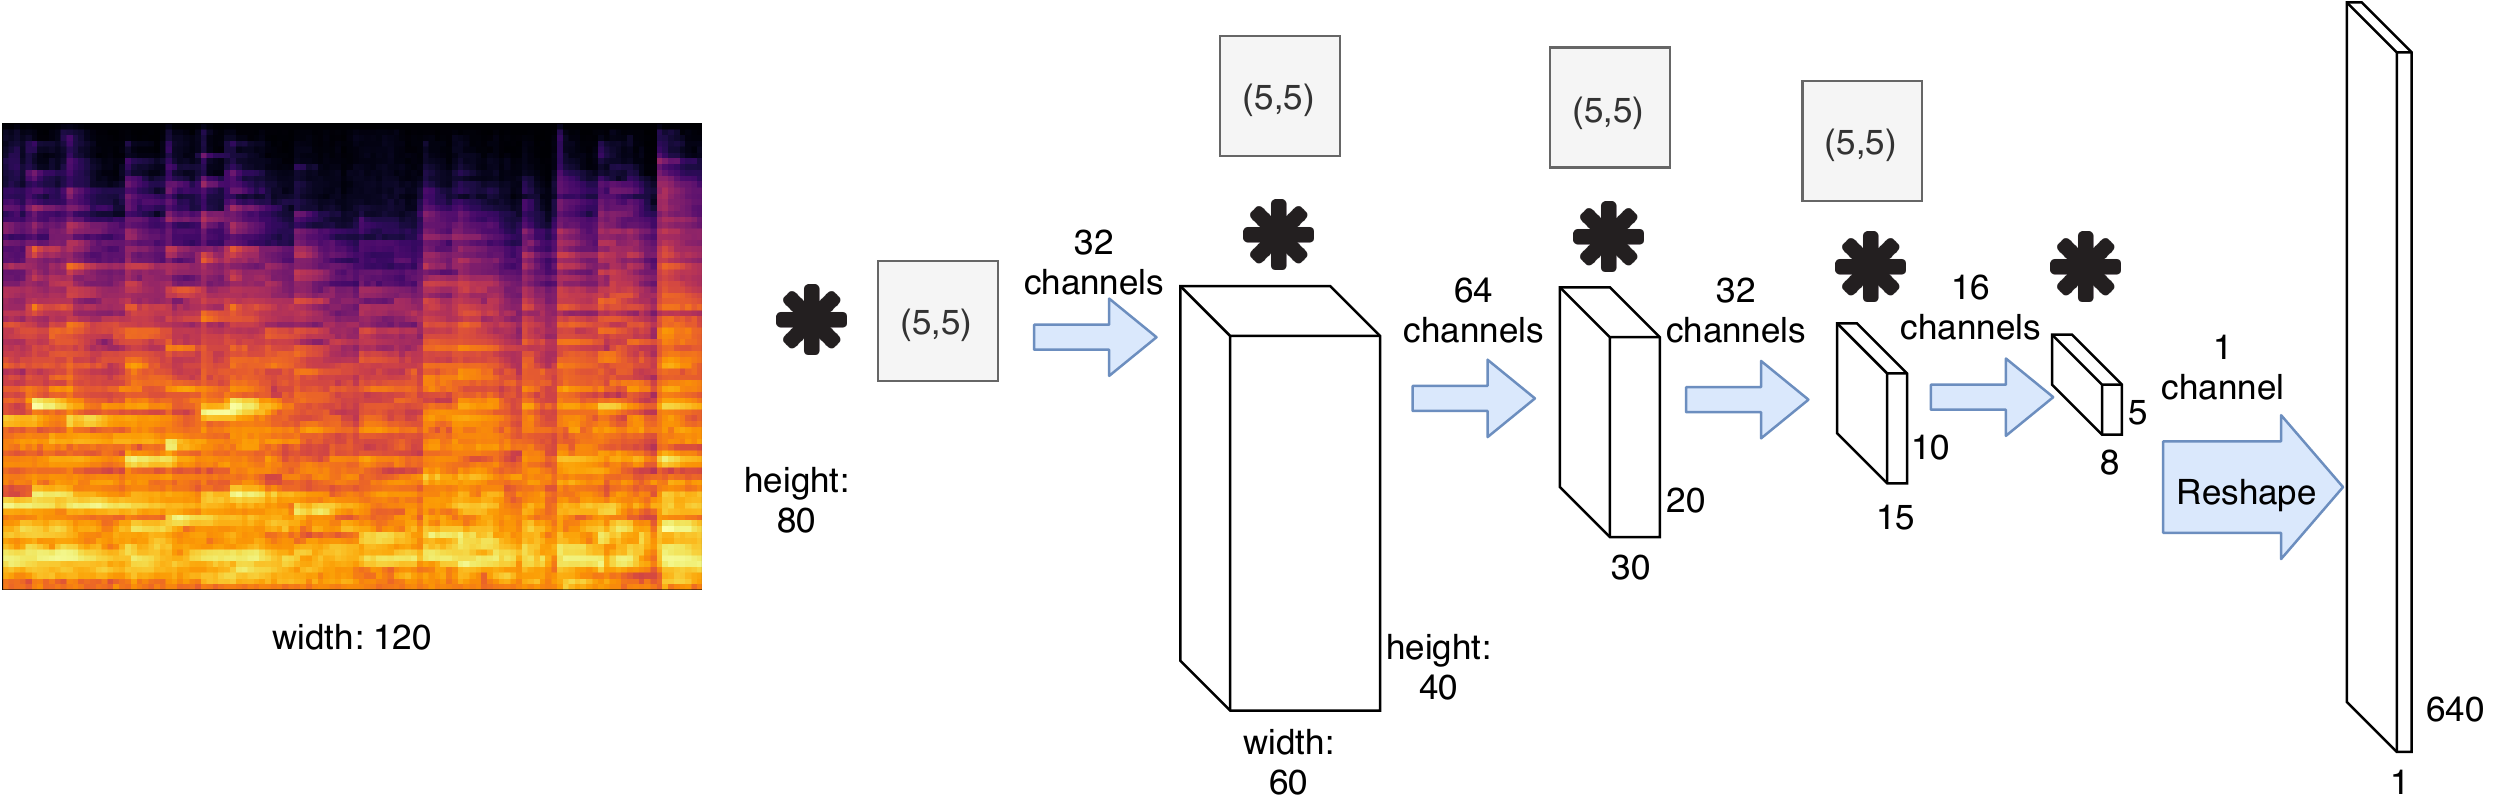}
	\caption{Detail of the encoder network.}
	\label{fig:encoder}
\end{center}
\end{figure*}

The general structure of the network can be seen on Fig. \ref{fig:overview-network}.

\begin{figure}[!th]
\begin{center}
	\includegraphics[width=\columnwidth]{audio-inpainting-gan-v6.pdf}
	\caption{(To be moved...) Overview of the GAN structure. \nicki{Can we simplify this? It looks crazy complicated, but actually isn't}\andi{I tried}}
\label{fig:overview-network}
 \end{center}
 \end{figure}

\subsection{Parameters}
	\label{subsec:params}

The signals used for training were all sampled at 22.05 kHz. For the listening tests, the signals were resampled to 48kHz. During training, the batch size was 64. For the `normal' condition tested on every dataset, the spectrograms were split into 480 time bins, 64 time bins and 480 time bins, equating to 5.6~s, 0.74~s and 5.6~s respectively. For the `short' condition, that split was 240, 32, and 240 and for the `long' condition it was 960, 128, and 960. 
% \andi{I think this next paragraph is already covered by Section III.B}

The generator's encoder consists of 4 convolutional layers with stride 2, filters of shape 5 by 5, and number of channels 32, 64, 32, and 16, respectively. The encoded signals is flattened before being processed by a liner layer with output size 8192. After, the signal is reshaped into a rectangle and processed by 4 convolutional layer with number of channels 256, 128, 64, 32, respectively. The first two filters have shape 4 by 4 after which all filters have shape 8 by 8. Then, the signal is processed by two 32 channels residual layers with filters shaped 8 by 8. Finally, there is one last convolutional layer with 1 channel as output. The discriminator is comprised of 2 networks processing STFT signals and 3 networks processing MEL signals. Both types of network follow the same basic structure with 5 layers each, using stride 2 for each layer and filters of size 5 by 5. The main difference was in the amount of channels where the networks processing STFT signals start with 32 channels and the networks processing MEL signals start with 8 channels. After that, both networks double the amount of channels with every layer.
